# Supplementary material for: Mitigating the Transition of SiV$^-$ in Diamond to an Optically Dark State
Source: arXiv:2512.06389 source file (2025-12-06)
Supplement: Supplementary file 1 [file SI.pdf]

# Supplementary Information: Mitigating the Transition of $SiV^-$ in Diamond to an Optically Dark State

Manuel Rieger,[1,2] Rubek Poudel,[1,2] Tobias Waldmann,[2,3] Lina M. Todenhagen,[1,2] Stefan Kresta,[2,3] Nori N. Chavira Leal,[2,3] Viviana Villafañe,[2,3] Martin S. Brandt,[1,2] Kai Müller,[2,3] Jonathan J. Finley[1,2]

[1]Walter Schottky Institute and School of Natural Sciences, Technical University of Munich, 85748 Garching, Germany
[2]Munich Center for Quantum Science and Technology (MCQST), 80799 Munich, Germany
[3]Walter Schottky Institute and School of Computation, Information and Technology, Technical University of Munich, 85748 Garching, Germany

(Dated: December 5, 2025)

## Supplementary Note 1 Stability of the initialized $SiV^-$ charge state of single emitters in the dark

Here, we assess the stability of the $SiV^-$ charge state at constant voltage in the dark, i.e. absence of laser illumination and in a cryostat shielding against room light. In other words, we will assess purely electrical effects of different voltages on the $SiV^-$ charge state. First, we initialize the single SiV center into its negative charge state using a green laser pulse. Then, we measure the intensity under resonant excitation after varying delays $\tau_1$. We assume that the $SiV^-$ photoluminescence intensity is proportional to the average fraction of time that the SiV is in its negative charge state.

Figure 1a shows a histogram recorded at 60 V where the delay time in the dark does not seem to affect the $SiV^-$ charge state population. However, Figure 1b shows the same histogram at 140 V and now longer delay times clearly reduces the average $SiV^-$ population. This is a sign of purely electrical charge state conversion of $SiV^-$ to a dark state.

To visualize the behavior for all voltages, Fig. 1c displays the initial intensity during the resonant readout pulse as a function of the delay time $\tau_1$ for each voltage. The $SiV^-$ population is stable versus $\tau_1$ for some voltages, increases for some and decreases for some. To understand the voltage-dependence better, Figure 1d shows the initial $SiV^-$ photoluminescence intensity as a function of the voltage. It is exactly the same data as in panel c, with reversed color bar and x-axis data. We see that up to and including 80 V, $I_{1,\mathrm{initial}}$ is independent of $\tau_1$. From 80 V to around 130 V, the intensity increases with $\tau_1$, indicating that a purely electrical effect converts SiV from the dark state to $SiV^-$. For voltages $> 130$ V, a purely electrical effect converts $SiV^-$ to the dark charge state, as indicated by the intensity decrease with $\tau_1$.

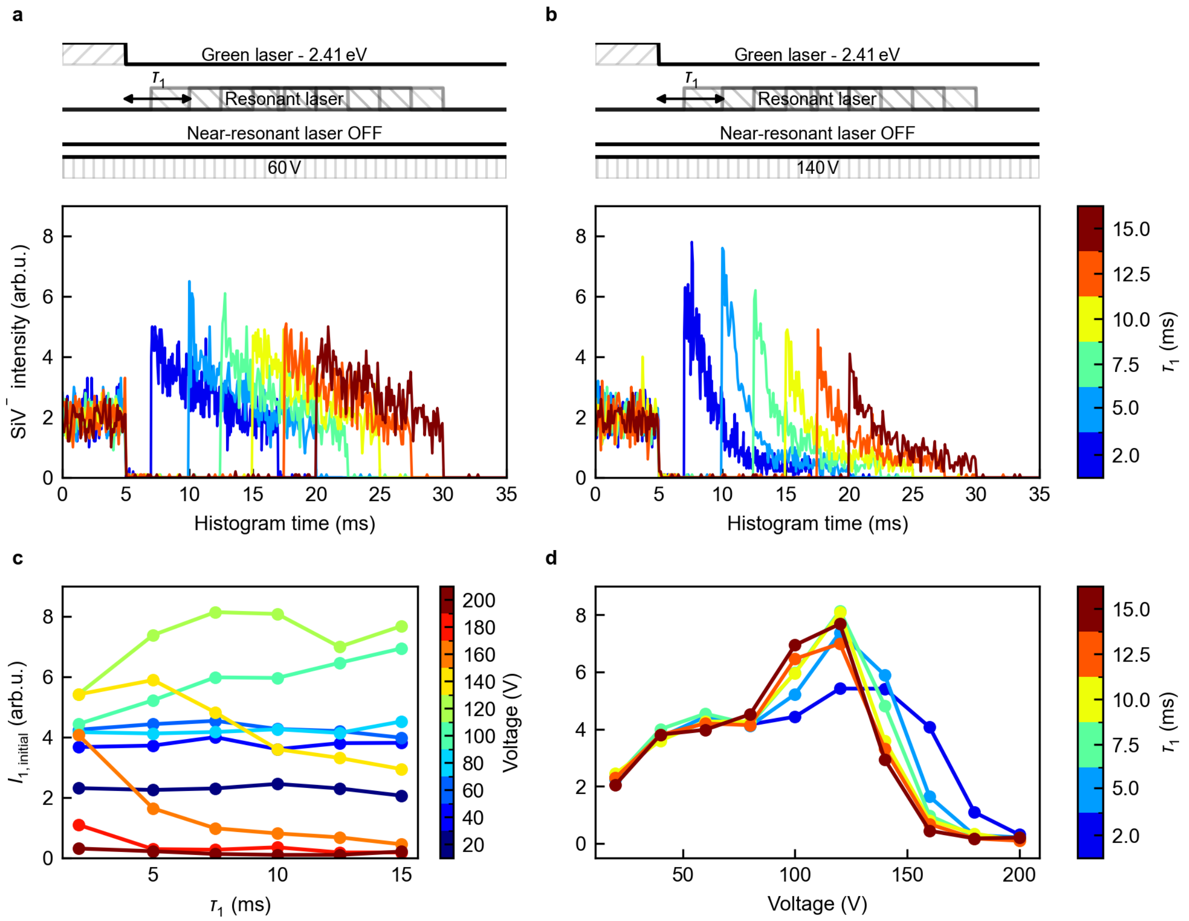


Supplementary Figure 1: **Stability of the SiV$^-$ charge state in the dark at different voltages.** We measure time-resolved photoluminescence of SiV$^-$ during a pulse sequence which consists of an initial 5 ms-long green laser pulse followed by a delay $\tau_1$ and then a 10 ms-long resonant readout pulse. **a** Histogram at 60 V. The initial intensity during resonant readout is mostly independent of $\tau_1$. **b** The same histogram but at 140 V. Now, the initial intensity clearly decreases with $\tau_1$. **c** The initial intensity during resonant excitation as a function of $\tau_1$. The color indicates the voltage. We see that some intensities increase, some decrease and some stay unchanged with $\tau_1$, depending on the voltage. **d** The initial SiV$^-$ photoluminescence intensity as a function of the voltage. Color indicates $\tau_1$. This is exactly the same data as in panel c, with reversed color bar and x-axis data. Up to and including 80 V, $I_{1,\mathrm{initial}}$ is independent of $\tau_1$. Afterwards and until around 130 V, the intensity increases with $\tau_1$. The highest voltages lead to a decrease of intensity with $\tau_1$.

# Supplementary Note 2 Additional time-resolved measurements with individual emitters

Here we present more time-resolved measurements of individual SiV like in the main text to provide some statistics. We did not perform the same type of measurement for emitters 1, 2 and 3, which we used only for test measurements, so we will start with emitter 4.

The plots show that certain emitters can be stabilized almost perfectly (emitters 4 and 5), while some emitters partially benefit from an applied voltage (emitters 7, 8 and 9) and others do not benefit at all (emitter 6). As discussed in the main text, we attribute these differences to locally varying parameters like strain and the types and distances to surrounding defects.

In Table 1, we present details on the voltage-dependent and time-resolved $SiV^-$ photoluminescence measurements shown in the main text (marked in bold) and on the on the analogous measurements presented in this section. The figures in this section depict the time integration windows used to calculate intensities $I_{ri}$ and $I_{rf}$. The figure of merit $I_{ri,max}/I_{ri}(0\,V)$ is the relative improvement of the initial count rate during the resonant excitation pulse. We see that a third of the emitters has an at least 3x improvement of this initial countrate when applying the optimal voltage, while a half shows moderate improvements and emitter 6 shows no improvement. Analogously, $I_{rf,max}/I_{rf}(0\,V)$ is the relative increase of the steady state count rate during resonant excitation. This figure of merit can be increased by a factor of 3 for two-thirds of the emitter, underlining the strong stabilizing effect caused by the applied voltage. The rest of the emitters also show an improvement. Note that these metrics are very conservative since we did not subtract the background intensity of the resonant laser, which would increase the values. Lastly, $I_{rf,max}/I_{ri,max}$ is a figure of merit that describes the relative stability of the steady-state countrate compared to the maximum initial countrate. Note that the optimal initialization and stabilization voltages are usually not the same, such that the overall efficiency would benefit from having different voltages during green laser initialization and resonant excitation. The best value is 0.97, which corresponds to only 3% relative loss of $SiV^-$ count rate/population during the 40 ms-long and strong resonant driving.

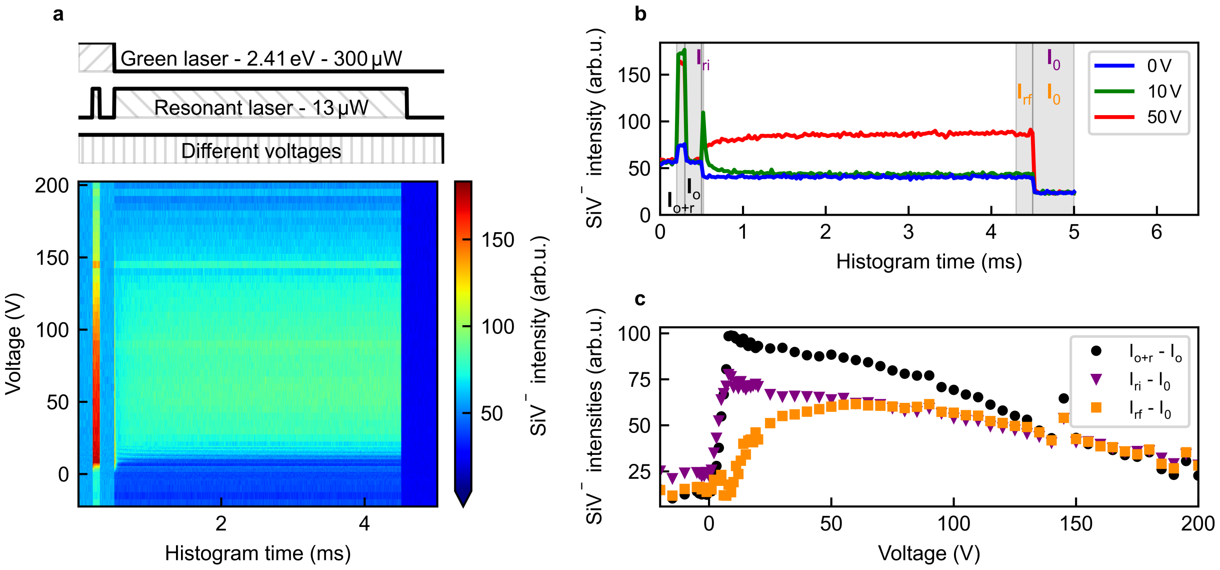


Supplementary Figure 2: **Time-resolved and voltage-dependent photoluminescence measurement of $SiV^-$ emitter 4.** Applying a voltage can massively improve $SiV^-$ charge state intialization. Additionally, voltages above 50 V stabilize the steady-state count rate at the level of the initial countrate.

Supplementary Table 1: Overview of measurement details and figures of merit for the time-resolved voltage-dependent measurements presented in this section.

| Emitter | Wavelength (nm) | Resonant power (µW) | Off-resonant power (µW) | Voltage range (V) | Histogram time range (ms) | $I_{\mathrm{ri,max}}/I_{\mathrm{ri}}(0\,\mathrm{V})$ | $I_{\mathrm{rf,max}}/I_{\mathrm{rf}}(0\,\mathrm{V})$ | $I_{\mathrm{rf,max}}/I_{\mathrm{ri,max}}$ |
|---|---|---|---|---|---|---|---|---|
| 4 | 737.086 | 13.0 | 302.0 | -20 to 200, 65 steps | 5 | 3.01 @8.0V | 3.8 @60.0V | 0.84 |
| **5** | **737.086** | **13.0** | **302.0** | **-200 to 200, 38 steps** | **50** | **4.12 @30.0V** | **4.58 @50.0V** | **0.97** |
| 5 | 737.086 | 126.0 | 302.0 | -200 to 200, 39 steps | 50 | 3.95 @40.0V | 4.13 @50.0V | 0.92 |
| 6 | 737.088 | 126.0 | 145.0 | -200 to 200, 72 steps | 50 | 1.0 @0.0V | 1.23 @13.0V | 0.22 |
| 7 | 737.087 | 126.0 | 145.0 | -1 to 200, 31 steps | 50 | 1.8 @1.0V | 3.0 @40.0V | 0.54 |
| 8 | 737.073 to 737.079, 28 steps | 126.0 | 121.0 | -190 to 180, 43 steps | 50 | 1.36 @25.0V | 3.01 @-190.0V | 0.43 |
| 9 | 737.075 to 737.083, 21 steps | 126.0 | 302.0 | -140 to 200, 35 steps | 50 | 1.74 @10.0V | 2.45 @20.0V | 0.35 |

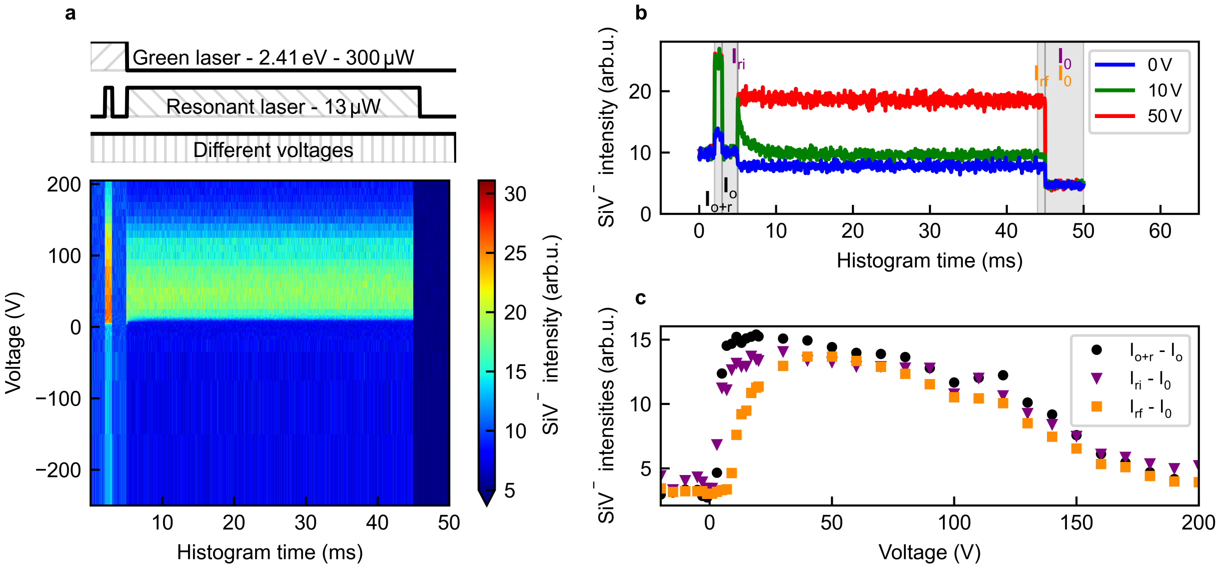


Supplementary Figure 3: **Time-resolved and voltage-dependent photoluminescence measurement of SiV$^-$ emitter 5.** This is the same emitter and the same measurement as in Fig. 2. The time integration windows for the intensities described in the main text are explicitly shown here.

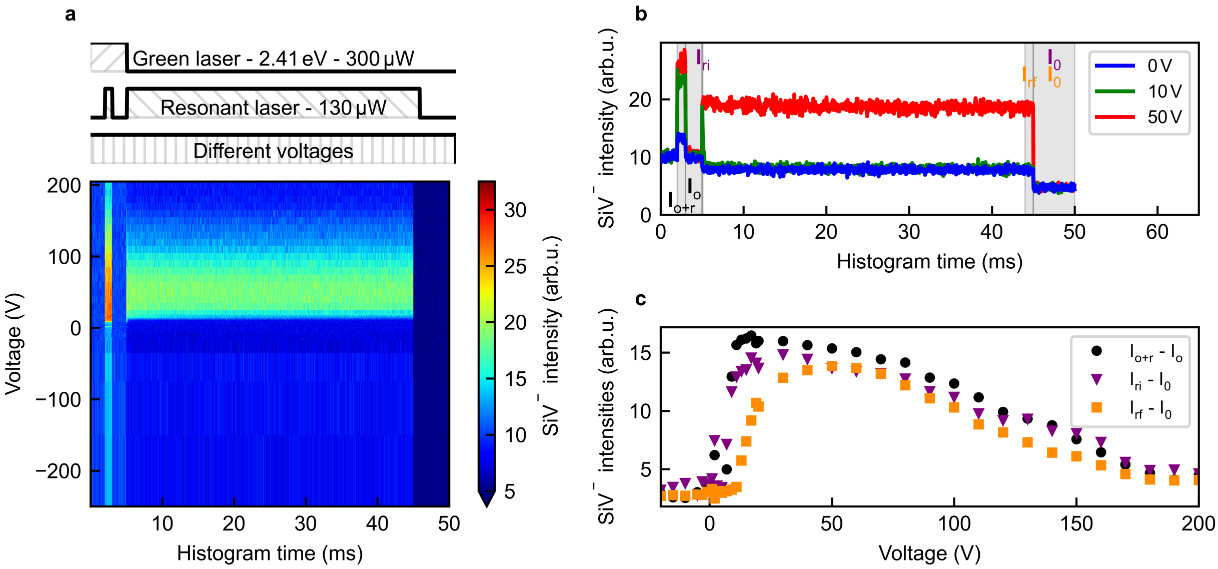


Supplementary Figure 4: **Time-resolved and voltage-dependent photoluminescence measurement of SiV$^-$ emitter 5.** This is the same emitter as in Fig. 2. We use a 10x higher resonant power now, which does not seem to make a big difference.

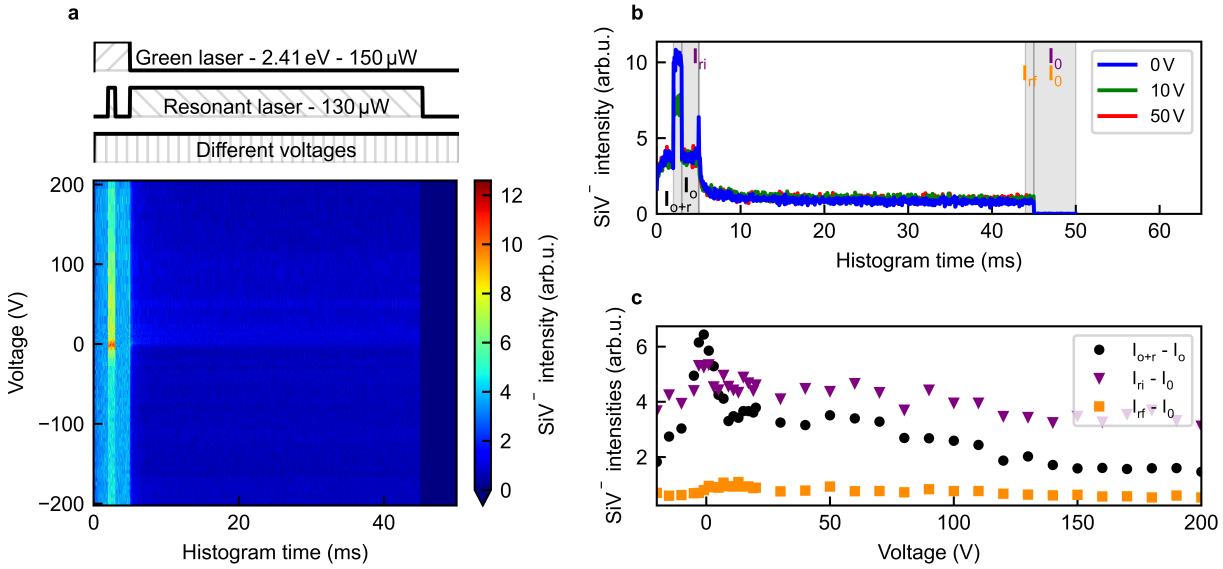


Supplementary Figure 5: **Time-resolved and voltage-dependent photoluminescence measurement of SiV$^-$ emitter 6.** This is an example where the bias voltage does not seem to stabilize the SiV$^-$ charge state. The initial intensity is the highest at 0 V and the voltage increases the steady state count rate only marginally.

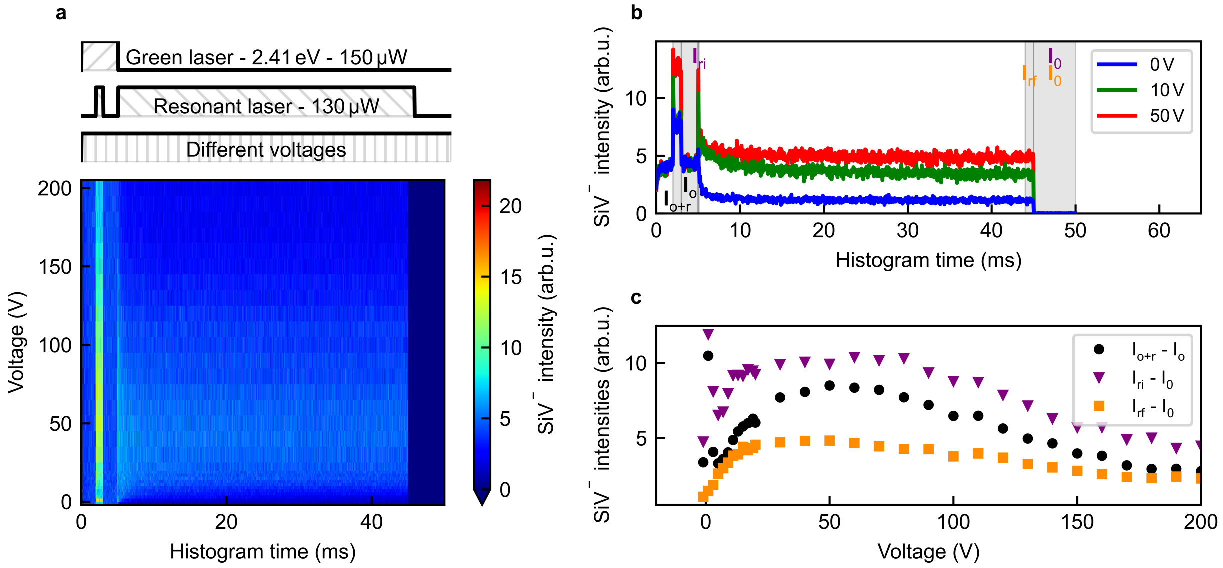


Supplementary Figure 6: **Time-resolved and voltage-dependent photoluminescence measurement of SiV$^-$ emitter 7.** This is an example where the bias voltage does not seem to improve the SiV$^-$ charge state initialization. The initial intensity is the highest at 0 V. However, the steady state count rate is practically zero at 0 V and massively increases by applying positive voltages.

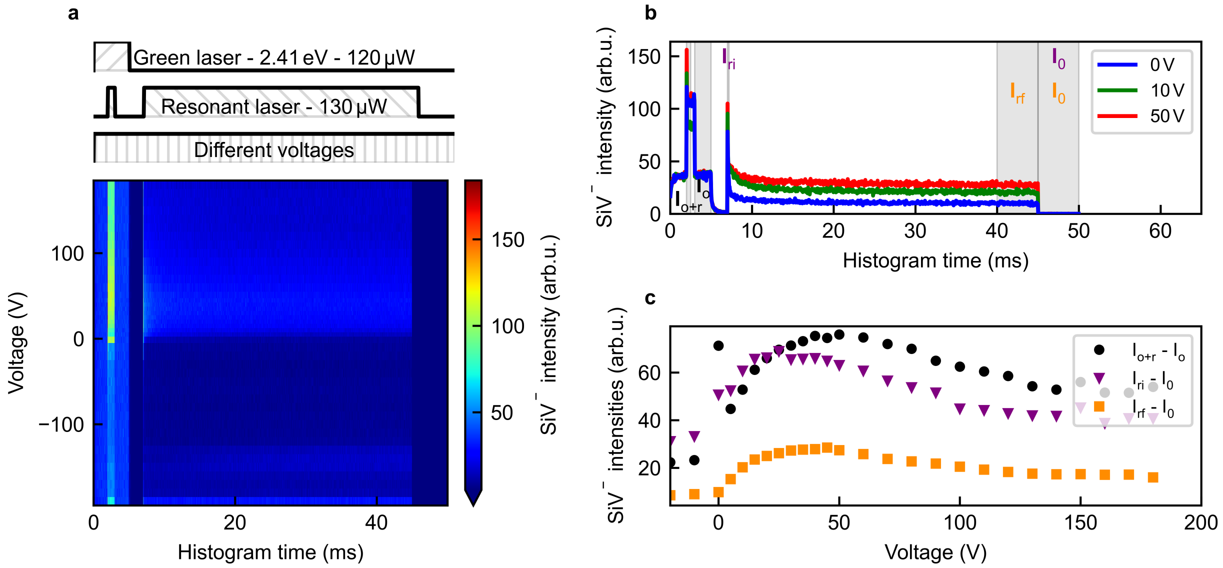


Supplementary Figure 7: **Time-resolved and voltage-dependent photoluminescence measurement of SiV$^-$ emitter 8, corrected for the Stark-shift of the transition.** To get the correct resonance laser frequency at each applied voltage, we first performed a separate measurement where we scanned the resonant laser over the optical resonance in voltage steps of $\leq 10\,\mathrm{V}$ and found a parabolic voltage-dependence of the resonance frequency. Below $-30\,\mathrm{V}$, we could not measure the resonances since initialization into SiV$^-$ did not work. At each voltage, we tuned the resonant laser to the parabolically fitted Stark-shifted resonance frequency. **b** We see that the steady-state count rate is significantly higher at 50 V, compared to 0 V. **c** The final resonant count rate as a function of voltage shows a relatively flat peak at 25 to 50 V while the initial resonant count rate has an optimum at slightly higher voltages from 30 to 70 V.

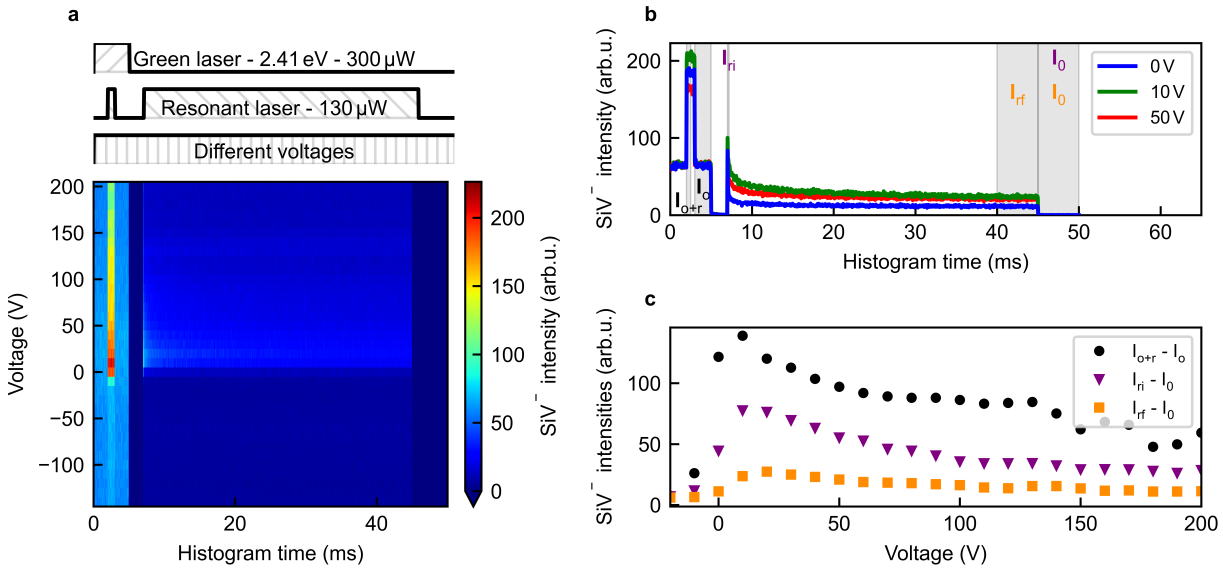


Supplementary Figure 8: **Time-resolved and voltage-dependent photoluminescence measurement of SiV$^-$ emitter 9.** We see that the bias voltage improves SiV$^-$ charge state initialization and stabilization during the resonant pulse.

## Supplementary Note 3 Voltage-dependent charge lifetime measurements with $SiV^-$ ensembles measured at two different points on the sample

In the main text, we primarily discuss measurements with single $SiV^-$ centers. However, section Supplementary Note 2 shows that there are differences between the individual centers. Here, we present measurements with $SiV^-$ center ensembles and assume that they allow us to estimate which fraction of $SiV^-$ centers can be stabilized using an applied voltage. The measurements are analogous to those in Fig. 2.

The top panel of Fig. 9a illustrates the pulse sequence used for these measurements. The resulting temporal $SiV^-$ photoluminescence histograms are plotted as a function of bias voltages ranging from −200 V to 200 V. We observe that negative biases close to the excitation spot result in a low resonant count rate during active stabilization and immediately afterwards, exactly as we observed it for the single emitter in the main text.

Figure 9b shows temporal traces for different voltages. The charge lifetimes for the ensemble do not exhibit significant variation; instead, the voltage primarily changes the initial count rate during resonant excitation and the steady state count rate at the end of the resonant pulse.

Figure 9c demonstrates that voltages from 0 to 20 V maximize the initial count rates. In contrast, the highest steady state count rate are achieved by applying 25 V. This indicates that an applied voltage can both improve charge initialization, as well as stabilize the the charge states of an $SiV^-$ center ensemble. The data indicate that there is a net positive effect on initialization and stabilization by the applied voltage.

Figure 10 presents the same type of measurement, repeated at another spot on the sample. The effects are qualitatively the same and we see a net improvement of the $SiV^-$ ensemble initialization and the steady state countrate.

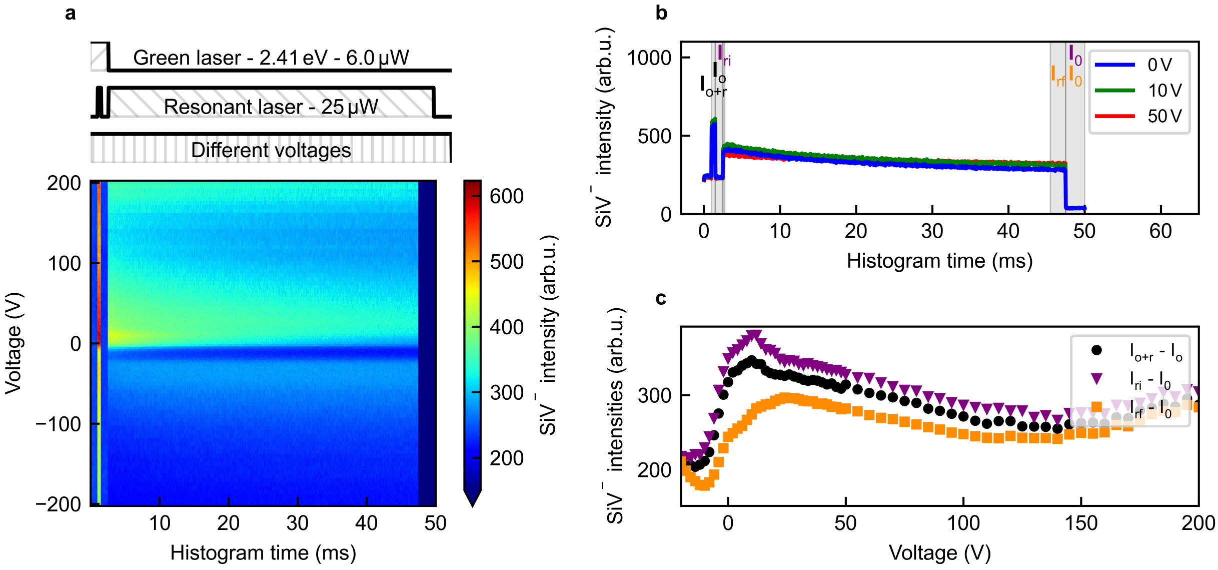


Supplementary Figure 9: **Time-resolved and voltage-dependent photoluminescence measurement of an $SiV^-$ ensemble.** **a** We again apply a pulse scheme with an off-resonant stabilization laser with a short resonant probe pulse, followed by a long resonant $SiV^-$ readout pulse. The wavelength was set to a maximum in photoluminescence excitation signal, measured at 20 V. **b** Temporal traces of the time-resolved $SiV^-$ intensity for selected voltages show an increased steady-state count rate at 10 V or 50 V compared to 0 V. **c** Different $SiV^-$ intensities as a function of bias voltage. The variables are marked in panel b. Applying 25 V strongly increases the steady-state count rate compared to 0 V, indicating $SiV^-$ charge state stabilization.

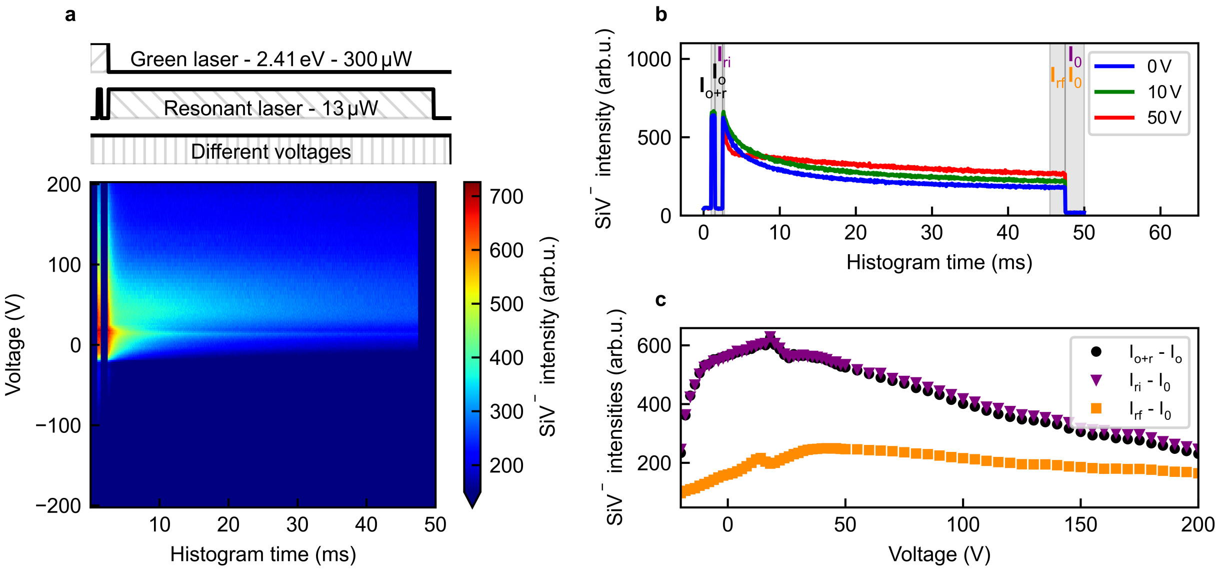


Supplementary Figure 10: **Time-resolved and voltage-dependent photoluminescence measurement of a second SiV$^-$ ensemble.**
